# Supplementary material for: Optical Spectrum of MoS${}_2$: Many-body Effects and Diversity of Exciton States
Source: arXiv:1311.0963 source file (2013-11-05)
Supplement: Supplementary file 1 [file Supplemental_Material.pdf]

# Supplemental Materials for "Optical Spectrum of $MoS_2$: Many-body Effects and Diversity of Exciton States"

Diana Y. Qiu, Felipe H. da Jornada, and Steven G. Louie*
*Department of Physics, University of California at Berkeley, California 94720 and*
*Materials Sciences Division, Lawrence Berkeley National Laboratory, Berkeley, California 94720*
(Dated: October 23, 2013)

## I. COMPUTATIONAL DETAILS

We perform our density functional theory (DFT) calculations in the local density approximation (LDA) using the QUANTUM ESPRESSO code[1]. The calculations are done in a supercell arrangement[2] with a plane-wave basis using normconserving pseudopotentials[3] with a 1700 eV wave function cutoff. We include the Mo semicore $4d$, $4p$, and $4s$ states as valence states for our DFT and GW-BSE calculations. The distance between repeated supercells in the out-of-plane direction is 25 Å. We fully relax the $MoS_2$ geometry, and the relaxed structure has an in-plane lattice constant of 3.15 Å, which deviates less than 1% from the experimental lattice constant of few layer $MoS_2$[4]. Spin-orbit interactions are included as a perturbation, which is discussed below.

When performing the GW and GW-BSE calculations with the BERKELEYGW package[5], we employ a truncated Coulomb potential[6] in order to eliminate spurious interactions between supercells in the out-of-plane direction. Slow convergence with respect to distance between repeated supercells has been suggested as a possible explanation for variations in the quasiparticle (QP) gaps across different GW calculations [7]. We note that our results are very close to the value of the $MoS_2$ QP gap extrapolated to infinite supercell size, in the absence of Coulomb truncation [7]. We take into account dynamical screening effects in the self-energy through the generalized plasmon pole model[8]. We also use Simple Approximate Physical Orbitals[9], for bands above $N_b$ = 2,400 bands, and the Static Remainder technique[10] to reduce the computational cost of generating a large number of unoccupied states.

## II. CONVERGENCE DETAILS

As discussed in the main text, we found the convergence of GW calculations on $MoS_2$ to be very sensitive to the number of empty bands included and the $(G, G')$ cutoff in the calculation of the dielectric matrix used for the screened interaction. On the Bethe-Salpeter level, however, we found that our calculation converged rather fast with the number of bands, with just 2 highest valence and 4 lowest conduction bands being sufficient. Going up to 7 valence and 8 conduction bands does not affect the optical spectrum up to $\omega \sim 3.5$ eV.

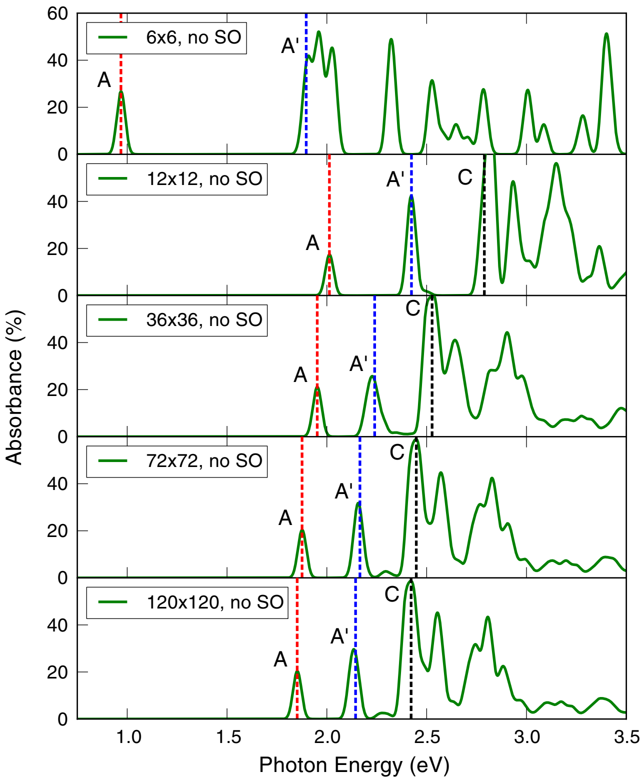


FIG. 1. (Color online) Convergence of the optical absorption spectrum with respect to the k-grid. For clarity, spin-orbit interactions are not included here in these test calculations. A gaussian broadening of 20 meV is applied to all spectra.

The convergence with the number of k-points, on the other hand, is much more complex and demanding, as shown in Fig. 1. The absorption spectrum changes qualitatively going from a 6x6x1 to a 12x12x1 grid, and the main features only start to converge on a 36x36x1 grid. Absolute peak positions are only converged on a 72x72x1 grid, and going further to a 120x120x1 grid shifts the first exciton peak (A) by less than 25 meV.

## III. SPIN-ORBIT INTERACTIONS

To account for the spin-orbit interaction in $MoS_2$, we take advantage of the facts that spin-orbit coupling splits the valence band maximum (VBM) but not the

* Email: sglouie@berkeley.edu

conduction band minimum (CBM) and spin is a good quantum number at the K and K' points[11]. We perform both a spin-unpolarized DFT calculation, which is used as the starting wave functions for our GW calculation, and a non-collinear calculation with spin-orbit interactions. We approximate the first-order spin-orbit correction to the GW quasiparticle energies to be the difference between the two Kohn-Sham split eigenvalues. That is, we take $\Delta\epsilon^{\rm SO}_{\rm GW}(n\mathbf{k}\sigma) \approx \Delta\epsilon^{\rm SO}_{\rm LDA}(n\mathbf{k}\sigma) \equiv \epsilon^{\rm non-col}(n\mathbf{k}\sigma) - \epsilon^{\rm unpol}(n\mathbf{k})$, where $\sigma$ is the spinor index of the states in the non-collinear calculation. This is a reasonable approximation since the overlaps between the spinor wave functions and the scalar wave functions are exactly 1 at $K$ and greater than 0.7 in other regions with spin-orbit splitting, in our LDA calculation.

To obtain the absorbance with spin-orbit interaction, we apply a first-order perturbation theory to the solution of the Bethe-Salpeter equation, which is justifiable because the quasiparticle gap ($\sim$ 2.8 eV) is much larger than the spin-orbit splitting ($\sim$ 150 meV). Each excitonic state $|S\rangle$ can be expanded as a linear combination of pairs of single-particle valence and conduction band states as

$$|S\rangle = \sum_{vc\mathbf{k}} A^S_{vc\mathbf{k}} \, |vc\mathbf{k}\rangle \, . \tag{1}$$

We want to calculate the spin-orbit corrected exciton energies $\Omega^S_\sigma = \Omega^S + \Delta\Omega^S_\sigma$, where $\Omega^S$ is the energy of the $|S\rangle$-state, neglecting spin-orbit, and $\Delta\Omega^S_\sigma$ is the first-order energy correction

$$\begin{aligned} \Delta\Omega^S_\sigma &\equiv \langle S|H^{\rm SO}_\sigma|S\rangle \\ &= \sum_{vc\mathbf{k}} \sum_{v'c'\mathbf{k}'} \left(A^S_{v'c'\mathbf{k}'}\right)^* A^S_{vc\mathbf{k}} \, \langle v'c'\mathbf{k}'|H^{\rm SO}_\sigma|vc\mathbf{k}\rangle \end{aligned} \tag{2}$$

where the spin-orbit Hamiltonian, $H^{\rm SO}$, is block-diagonal in the spin-index $\sigma$ and $H^{\rm SO}_\sigma$ is a block of the spin-orbit Hamiltonian for the spin $\sigma$. We assume that $H^{\rm SO}_\sigma$ is diagonal in the $|vc\mathbf{k}\rangle$ basis, which is valid due to the large overlap between the spinor and scalar wave functions. Then, the spin-orbit correction to the excited-state energies becomes

$$\Delta\Omega^S_\sigma = \sum_{vc\mathbf{k}} |A^S_{vc\mathbf{k}}|^2 \Delta\epsilon^{\rm SO}_{vc\mathbf{k}\sigma} \tag{3}$$

where $\Delta\epsilon^{\rm SO}_{vc\mathbf{k}\sigma}$ are the spin-orbit corrected differences in energy between the valence and conduction states

$$\begin{aligned} \Delta\epsilon^{\rm SO}_{vc\mathbf{k}\sigma} = &\left(\epsilon_{\rm GW}(c\mathbf{k}) + \Delta\epsilon^{\rm SO}_{\rm GW}(c\mathbf{k}\sigma)\right) \\ &- \left(\epsilon_{\rm GW}(v\mathbf{k}) + \Delta\epsilon^{\rm SO}_{\rm GW}(v\mathbf{k}\sigma)\right) \end{aligned} \tag{4}$$

Finally, the imaginary part of the dielectric function with spin-orbit interactions is calculated using the spin-orbit corrected exciton energies

$$\epsilon_2(\omega) = \frac{16\pi^2 e^2}{\omega^2} \sum_{S\sigma} |\mathbf{e} \cdot \langle 0|\, \mathbf{v} \,|S\sigma\rangle\, |^2 \delta(\omega - \Omega^S_\sigma) \tag{5}$$

where $\mathbf{e}$ is the polarization of the incoming light, $\mathbf{v}$ is the velocity operator, and $|S\sigma\rangle = |S\rangle$.

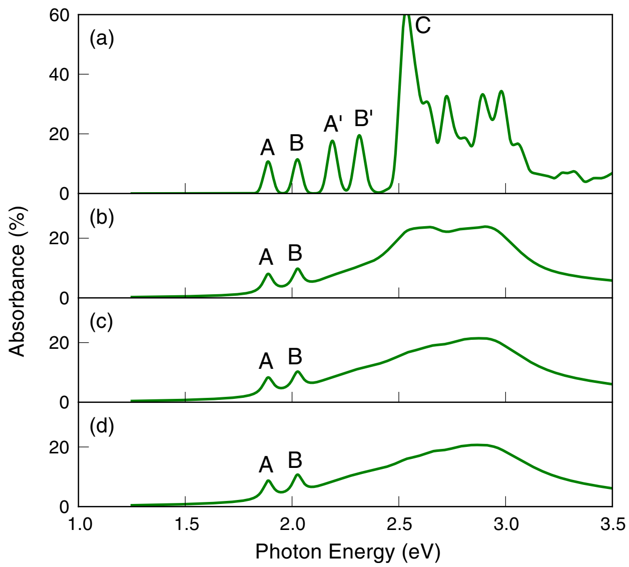


FIG. 2. Comparison of different broadening schemes for the calculated optical absorption spectrum. (a) Constant Gaussian broadening of $\sigma$ = 20 meV. (b-d) State-dependent broadening[12] using scattering rates of quasiparticle from *ab initio* electron-phonon interactions[13]. : (b) constant extrapolation, (c) linear extrapolation, (d) quadratic extrapolation.

## IV. INCLUSION OF QUASIPARTICLE LIFETIMES

We include the broadening due to quasiparticle lifetime in our calculation from first principles following the approach from Ref. [12], and we consider both absorption and emission of phonons at $T$ = 300 K. The carrier lifetimes due to electron-phonon interactions are taken from Ref. [13], which only reports quasi-electron scattering rates, and for quasiparticle energies $\epsilon(\mathbf{k})$ up to $\sim$ 0.25 eV, measured with respect to the conduction band minimum. In this work, we assume the quasi-hole scattering rate to be the same as the quasi-electron, and we further linearly extrapolate the quasiparticle lifetimes for carrier energies larger than $\sim$ 0.25 eV above the CBM. In Figure 2 (b-d), we compare the resulting absorption spectrum obtained from this linear extrapolation with a constant and quadratic extrapolation of the scattering rate. A more rigorous solution would involve calculating the wave vector-dependent scattering rate in the full Brillouin zone for a few conduction and valence bands, but it is beyond the scope of this work.

## V. EXCITON SPECTRUM

As mentioned in the main discussion, although we use the notation of the 2D hydrogen model (e.g. 1s, 2s, 2p) to refer to the optically excited states, our GW-BSE exciton spectrum is completely different from that of a 2D

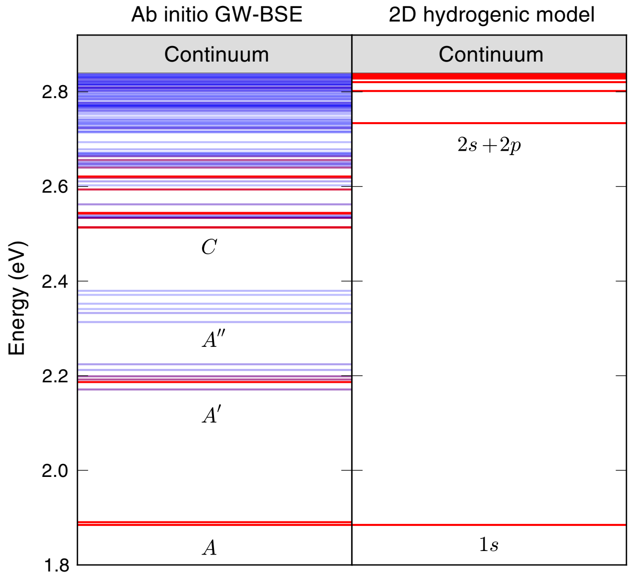


FIG. 3. (Color online) Comparison of the exciton state energy levels obtained from our *ab initio* GW-BSE calculation (left) with an effective 2D hydrogenic atom (right). Bright [dark] exciton states are represented by opaque red [transluscent blue] lines.

hydrogenic model. In Fig. 3, we compare the exciton energy levels from our GW-BSE calculation with the exciton spectrum from a 2D hydrogenic model with the calculated quasiparticle band masses and an effective dielectric constant fit to the binding energy of state A. The binding energies of the other excitons in our calculation (A', A", etc.) are much larger than the energies predicted from the 2D hydrogenic model, which does not account for spatial variation in the dielectric function. A similar enhancement of binding energies of excited states of excitons due to large $q$-dependent screening (which leads to anti-screening effects) has been seen in other low-dimensional systems, such as in carbon nanotubes[14].


[1] P. Giannozzi, S. Baroni, N. Bonini, M. Calandra, R. Car, C. Cavazzoni, D. Ceresoli, G. L. Chiarotti, M. Cococcioni, I. Dabo, A. D. Corso, S. de Gironcoli, S. Fabris, G. Fratesi, R. Gebauer, U. Gerstmann, C. Gougoussis, A. Kokalj, M. Lazzeri, L. Martin-Samos, N. Marzari, F. Mauri, R. Mazzarello, S. Paolini, A. Pasquarello, L. Paulatto, C. Sbraccia, S. Scandolo, G. Sclauzero, A. P. Seitsonen, A. Smogunov, P. Umari, and R. M. Wentzcovitch, J. Phys.: Condens. Matt. **21**, 395502 (2009).

[2] M. L. Cohen, M. Schlüter, J. R. Chelikowsky, and S. G. Louie, Phys. Rev. B **12**, 5575 (1975).

[3] N. Troullier and J. L. Martins, Phys. Rev. B **43**, 1993 (1991).

[4] P. A. Young, J. Phys. D Appl. Phys. **1**, 936 (1968).

[5] J. Deslippe, G. Samsonidze, D. Strubbe, M. Jain, M. L. Cohen, and S. G. Louie, Comput. Phys. Commun. **183**, 1269 (2012).

[6] S. Ismail-Beigi, Phys. Rev. B **73**, 233103 (2006).

[7] H.-P. Komsa and A. V. Krasheninniko, Phys. Rev. B **86**, 241201 (2012).

[8] M. S. Hybertsen and S. G. Louie, Phys. Rev. B **34**, 5390 (1986).

[9] G. Samsonidze, M. Jain, J. Deslippe, M. L. Cohen, and S. G. Louie, Phys. Rev. Lett. **107**, 186404 (2011).

[10] J. Deslippe, G. Samsonidze, M. Jain, M. L. Cohen, and S. G. Louie, Phys. Rev. B. **87**, 165124 (2013).

[11] D. Xiao, G.-B. Liu, W. Feng, X. Xu, and W. Yao, Phys. Rev. Lett. **108**, 196802 (2012).

[12] A. Marini, Phys. Rev. Lett. **101**, 106405 (2008).

[13] X. Li, J. T. Mullen, Z. Jin, K. M. Borysenko, M. Buongiorno Nardelli, and K. W. Kim, Phys. Rev. B **87**, 115418 (2013).

[14] J. Deslippe, M. Dipoppa, D. Prendergast, M. V. O. Moutinho, R. B. Capaz, and S. G. Louie, Nano Lett. **9**, 1330 (2009).
